# Supplementary material for: Markov Stochastic Choice
Source: arXiv:2410.22001 source file (2024-10-29)
Supplement: Supplementary file 1 [file app-3-luce.tex]

\subsection{Proof of Proposition~\ref{prop:luce}}
\label{proof:luce}
\textit{Necessity}: Let $\mat{\M}$ be a reversible \msc[l] with strictly positive transition probabilities between all pairs of alternatives. Fix a menu $\M\in\Mset$ and a pair $i,j\in\M$. We will show that positivity and IIA hold for this pair and hence, for all other pairs and menus. 

Since the transition probabilities between all pairs are strictly positive, the stationary distributions are such that $\ro[]{}{i}{\M}>0$ for all $i\in\M$ and all $\M\in\Mset$. Hence, the induced stochastic choice function is positive. Reversibility implies that 
\[\frac{\ro[]{}{i}{\M}}{\ro[]{}{j}{\M}}=\frac{\q{ji}{}}{\q{ij}{}} \text{  and  }\frac{\ro[c]{}{i}{i,j}}{\ro[c]{}{j}{i,j}}=\frac{\q[c]{ji}{i,j}}{\q[c]{ij}{i,j}}.\]
Because of TR-IIA all fractions in the above equations are equal and hence IIA is satisfied.

\textit{Sufficiency}: Let \bp[]{} be a positive stochastic choice function that satisfies IIA, that is
\begin{equation*}
\p[c]{j}{i,j}\p{i}{\M}=\p[c]{i}{i,j}\p{j}{\M},\quad \forall i,j\in\M, \forall \M\in\Mset.
\end{equation*}
%\label{eq:revers-bin}
Note that $\dif{ji}{}=\p{j}{\M}-\frac{\p[c]{j}{i,j}}{\p[c]{i}{i,j}}\p{i}{\M}=0$ for all $i,j\in\M$. Lemma~\ref{lem3} in Appendix~\ref{app-gen} implies that the stochastic choice function is rationalizable by a \msc[l] with strictly positive transition probabilities. We will show that all such rationalizing models are reversible, hence 
\begin{equation*}
\q{ij}{}\p{i}{\M}=\q{ji}{}\p{j}{\M},\quad \forall i,j\in\M, \forall \M\in\Mset.
\end{equation*}
We apply IIA and Example~\ref{exp-binary} and obtain
\begin{equation*}
\frac{\p{j}{\M}}{\p{i}{\M}}=\frac{\p[c]{j}{i,j}}{\p[c]{i}{i,j}}=\frac{\q[c]{ji}{i,j}}{\q[c]{ij}{i,j}}.
\end{equation*}
Finally, TR-IIA and the above equation imply that
\begin{equation*}
\q{ij}{}\p{i}{\M}=\q{ji}{}\p{j}{\M}.
\end{equation*}
Therefore, detailed balance holds on all pairs and menus and the rationalizing model is reversible for all menus.
\subsection{Proof of Corollary~\ref{cor:utility}}
\label{proof:utility}
\textit{Necessity}: If there exists a utility function such that the ratios of transition probabilities satisfy equation~\eqref{eq:ratio-utility}, reversibility of the \msc[l] is trivial as it follows directly from Kolmogorov's criterion.

\textit{Sufficiency}: Let \mat{\M} be a reversible \msc[l] with strictly positive transitions. In Proposition~\ref{prop:luce} we show that the model is characterized by IIA and positivity. Therefore, a stochastic choice function generated by the \msc[l] $\mat{\M}$ is a Luce rule. Hence, there exists an increasing function ${u:\all\rightarrow \mathbb{R}_{++}}$ such that for all $\M \in \Mset$ and $i\in \M$ such that
\[\p{i}{\M}=\frac{\val{i}}{\sum_{j\in \M} \val{j}}. \]
Since the model is reversible, it satisfies detailed balance on each pair of alternatives. Hence, it holds for all $i,j \in\M$ and all $\M\in\Mset$ that
\begin{equation*}
\begin{gathered}
\q{ji}{}\p{j}{\M}=\p{i}{\M}\q{ij}{}\\
\q{ji}{}\frac{\val{j}}{\sum_{k\in \M} \val{k}}=\frac{\val{i}}{\sum_{k\in \M} \val{k}}\q{ij}{}
\end{gathered}
\end{equation*}
and the result follows.
