# Supplementary material for: Markov Stochastic Choice
Source: arXiv:2410.22001 source file (2024-10-29)
Supplement: Supplementary file 2 [file app-4-edge.tex]

\subsection{Proof of Proposition~\ref{prop:no-edges}}
\label{proof:no-edges}
Let $\bp{}$ be a stochastic choice function rationalizable by a \msc[l] $\mat{\M}$ which is positive on binary choice sets and it holds for at least one pair $i,j\in\M$ that the choice over the pair is not\btc{}. This implies that $i\spo j$ w.l.o.g.\ and there is no cycle \cy such that $(i,j)\in\cy$. Similarly to the proof of Theorem~\ref{t:reversible}, we will use the function $\dif{}{}$ defined in Appendix~\ref{app-gen}, which is always defined because $\bp{}$ is positive on binary sets. Note that $i\spo j$ implies $\dif{ji}{}>0$. We assume by contradiction that there is a rationalizing model $\mat{\M}$ with $\q{ij}{}>0$. Because of TR-IIA it holds also that $\q{ji}{}>0$.  
%As shown in Theorem~\ref{t:reversible} applying Gordan's theorem implies that the system
%%  \begin{equation}
%%	\mathcal{D}(\M)\sav{}=\boldsymbol{0}
%%	\end{equation}
%has a strictly positive solution if \spo is cyclical and no strictly positive solution if \spo is acyclical. Hence, if \spo is acyclical, $\q{ij}{}=0$, which is a contradiction.
Since $\bp{}$ violates the\btc{c}, it follows from Theorem~\ref{t:all} that there has to be at least one pair $k,l\in\M$ for which $\dif{kl}{}\neq 0$ and $\q{kl}{}=0$. 

Since $\spo\neq\emptyset$, we define the set $\G$ and the functions $f_{\M}(.)$, $\g[.]$, and a matrix $\mathcal{D}(\M)$ in the same way as we do in the sufficiency proof of Theorem~\ref{t:reversible} (see Appendix~\ref{proof:theorem-reversible}). Let w.l.o.g.\ that $(i,j)\in\G$ and $\mathcal{P}(\G)$ denote the power set of $\G\setminus (i,j)$ with characteristic element $\mathcal{G}$.

We show the contradiction by constructing stochastic choice functions $\bp{}'$ from $\bp{}$ for each set in $\mathcal{P}(\G)$ by adjusting $\p[c]{k}{k,l}$ such that $\dif{kl}{}'=0$ for all $(k,l)\in \mathcal{G}$, for all $\mathcal{G}\in \mathcal{P}(\G)$. What this means is that $\G'\subset\G$ and that $\sav{}'$ has less dimensions than $\sav{}$. Among those stochastic choice functions there needs to be one, say $\bp{}^*$, in which exactly those pairs of alternatives are excluded from $\G^*$ for which there is zero transition probability in $\mat{\M}$, that is, for all $k,l\in\M$ for which $\q{kl}{}=0$ and $(k,l)\in\G$ holds that $(k,l)\not\in\G^*$ and $\dif{kl}{}^*=0$, and for all $k,l\in\M$ for which $\q{kl}{}>0$ and $(k,l)\in\G$ holds that $(k,l)\in\G^*$. 

Let $\mat{\M}^*$ be such that $\q{mn}{}^*=\q{mn}{}$ for all $m,n\in\M$ for which ${\q{mn}{}>0}$ and $\q{mn}{}^*\in(0,1)$ and $\q{nm}{}^*=\q{mn}{}^*\frac{\p[c]{m}{m,n}^*}{\p[c]{n}{m,n}^*}$ for all $m,n\in\M$ for which $\q{mn}{}=0$. In particular, since ${\q{ij}{}>0}$, $\q{ij}{}^*=\q{ij}{}$. Due to the way $\bp{}^*$ is constructed from $\bp{}$, the choice over the pair $i,j$ according to $\bp{}^*$ is not\btc{}. 

The constructed \msc[l] rationalizes $\bp{}^*$ and has strictly positive transition probabilities. Theorem~\ref{t:all} implies that all pairs of alternatives are\btc{}. However, the pair $i,j$ violates the condition, which is a contradiction. Therefore, we must have $\q{ij}{}=0$.
