# Supplementary material for: Markov Stochastic Choice
Source: arXiv:2410.22001 source file (2024-10-29)
Supplement: Supplementary file 3 [file app-4-ergodic.tex]

\subsection{Proof of Theorem~\ref{t:ergodic}}
\label{proof:theorem-ergodic}

\textit{Necessity}: Let $\mat{\M}$ be an ergodic \msc[l]. Hence, for each menu~$\M$ there is a sequence of alternatives~$I(\M)$ such that it holds for all consecutive elements $(i,j)$ that $\q{ij}{}>0$. We want to show that the generated stochastic choice function is positive on binary sets and that for all subsequent pairs of alternatives in $I(\M)$ it holds that the induced choice over the pair is\btc{}. 

The positivity of the stochastic choice function on binary sets is an immediate consequence of the irreducibility of the Markov chain. Note that irreducibility on binary menus requires that $\q[c]{ij}{i,j}\in (0,1)$ for all $i,j\in\all$. 
%TR-IIA then implies that for all $\M\in\Mset$ and all $i,j\in\M$ we either have ${\q{ij}{}>0},{\q{ji}{}>0}$ or $\q{ij}{}=\q{ji}{}=0$. This result combined with the irreducibility of the Markov chain imply that for each menu $\M\in\Mset$ there exists some sequence of the elements in the menu such that $\q{ij}{}>0$ and $\q{ji}{}>0$ for all consecutive elements $i,j$ in the sequence. 

We now need to show that it holds for all consecutive pairs in $I(\M)$ that the generated choice is\btc{}. Assume by contradiction that this is not the case for some pair $i,j$. Then, $i\spo j$, but there is no cycle $\cy$ for which $(i,j)\in\cy$. Proposition~\ref{prop:no-edges} then implies that all rationalizable models of \brho{} are such that $\q{ij}{}=\q{ji}{}=0$, which is a contradiction.
%If the detailed balance condition holds between some consecutive elements of the sequence $i,j$, therefore ${\ro[]{}{i}{\M}\q{ij}{}=\ro[]{}{j}{\M}\q{ji}{}}$. TR-IIA then implies that $\ro[]{}{i}{\M}\ro[c]{}{j}{i,j}=\ro[]{}{j}{\M}\ro[c]{}{i}{\M}$ and hence $\dif{ij}{}=0$. 
%
%Consider now the consecutive pairs in the sequence for which detailed balance is violated. Analogously, the generated stochastic choice function is such that $\dif{ij}{}\neq 0$ for all such pairs $i,j$. Assume by contradiction that $i,j$ do not belong to any cycle of \spo. Let $\brho{}=\bp[n]{\M}$.  Hence, it holds for all consecutive pairs of the sequence for which $\dif{ij}{}\neq 0$ that they belong to some cycle of $\spo$.

\textit{Sufficiency}: Let $\bp{}$ be a stochastic choice function which is positive on binary choice sets and for which there is a sequence of the alternatives in the menu $I(\M)=(i,j,\dots)$ (possibly with repetitions) such that all consecutive pairs $(i,j)$ are\btc{}. We will first show that the rationalizing model is such that for all $\M\in\Mset$ and $i,j\in\M$ it holds that either ${\q{ij}{}>0},{\q{ji}{}>0}$ or $\q{ij}{}=\q{ji}{}=0$. Then, we will show that there exists an irreducible \msc[l], in particular that for all consecutive elements in the above sequence the transition probability is strictly positive. Since \msc[l]s are aperiodic by definition, proving irreducibly implies that the \msc[l] is ergodic.

Suppose that there is a rationalizing \msc[l] with $\q{ij}{}>0$ and $\q{ji}{}=0$. Since $\bp{}$ is positive on binary choice sets, we must have $\q[c]{ij}{i,j}>0$ and $\q[c]{ji}{i,j}>0$. Under these assumptions, TR-IIA is violated and we have found a contradiction.

We now show the existence of a \msc[l] with strictly positive transitions between every two consecutive alternatives in~$I(\M)$. We start by constructing a stochastic choice function $\bp[]{\M}'$ from $\bp[]{\M}$, where we adjust $\p[c]{k}{k,l}$ for all $k\spo l$ that are not\btc{} such that $\dif{kl}{}'=0$. Note that the constructed stochastic choice function $\bp[]{\M}'$ has to satisfy the\btc{m} on all pairs $i,j\in\M$. It also satisfies positivity on binary sets because we assume it for $\bp[]{\M}$.

Theorem~\ref{t:all} implies that $\bp[]{\M}'$ is rationalizable with a \msc[l] $\mat[']{\M}$ with only strictly positive transitions. Now let $\mat{\M}$ be such that $\q{ij}{}=\q{ij}{}'$ for all pairs $i,j$ that are\btc{} and $\q{ij}{}=\q{ji}{}=0$ for all $i,j$ that are not\btc{}. The constructed matrix~$\mat{\M}$ satisfies equation~\eqref{eq:diff} and hence rationalizes the stochastic choice function $\bp[]{\M}$. Since we only adjust the transition probability between pairs of alternatives that do not belong to the sequence $I(\M)$, in the constructed model the transition probabilities between the subsequent elements of $I(\M)$ are strictly positive. Since the sequence spans over the whole menu, the constructed Markov chain is ergodic.
