# Supplementary material for: Markov Stochastic Choice
Source: arXiv:2410.22001 source file (2024-10-29)
Supplement: Supplementary file 4 [file app-4-time.tex]

\subsection{Proof of Proposition~\ref{prop:initial}}
\label{proof:initial}
Fix a menu $\M\in\Mset$ and let $\brhod[d]{i}$ denote the stochastic choice function generated by the \msc[b] with initial distribution equal to the degenerate distribution with point mass on alternative~$i$. 
	We will first show that a stochastic choice function is a linear combination of the stochastic choice functions from degenerate initial conditions. Let ${V=(I-(1-\abs)\mat[]{\M})}$ and ${W=V^{-1}}$, which exists for $\abs \neq 0$. Recall from equation~\eqref{eq-def} that
	\begin{align*}
	\brhod[]{}&= \abs \init{}{} (I-(1-\abs)\mat[]{\M})^{-1}=\abs \init{}{}V^{-1}=\abs \init{}{}W. 	
	\end{align*}
Since we have fixed $\abs$ and $\mat[]{\M}$ we will use the following simplified notation to denote the probability to choose alternative $i$ from the menu $\rod{i}{\init[]{}}=\rode{i}{\boldsymbol{\pi}}$. 

Note that $\rode{i}{\delta_j}=\abs w_{ji}$ for any $i,j\in \M$. If $\init{}{}$ is not degenerate, we have that 
\begin{equation}
\label{deg-sum}
\rode{i}{\boldsymbol{\pi}}=\sum_{j\in \M}\init[j]{}\abs w_{ji}=\sum_{j\in \M}\init[j]{} \rode{i}{\delta_j}\quad \forall i\in\M.
\end{equation}
	Let $i$ be the target alternative. We will now show that ${\rode{i}{\delta_i}> \rode{i}{\delta_j}}$ for all $j\neq i$. Denote ${\max_{j\neq i}\{\rode{i}{\delta_j}\}=\rode{i}{\delta_m}}$. Since $V\cdot W=I$ we obtain the following equation when we multiply $V$'s $m^\text{th}$ row vector with $W$'s $i^\text{th}$ column vector:
	\begin{equation*}
	\begin{gathered}
		(1-(1-\abs)\q{mm}{})w_{mi}+\sum_{j \neq m}(-1)(1-\abs)\q{mj}{}w_{ji}=0\\
	(1-(1-\abs)(1-\sum_{j\neq m}\q{mj}{}))w_{mi}-(1-\abs)\sum_{j \neq m}\q{mj}{}w_{ji}=0\\
		(\abs+(1-\abs)\sum_{j\neq m}\q{mj}{})w_{mi}-(1-\abs)\sum_{j \neq m}\q{mj}{}w_{ji}=0\\
		(1-\abs)(\sum_{j\neq m}\q{mj}{}(w_{ji}-w_{mi}))=\abs w_{mi}
				\end{gathered}
	\end{equation*}
Finally, we plug in $\rode{i}{\delta_j}=\abs w_{ji}$ and obtain
	\begin{equation*}
	\begin{gathered}
		\sum_{j\neq m}\q{mj}{}(\rode{i}{\delta_j}-\rode{i}{\delta_m})=\frac{\abs}{1-\abs} \rode{i}{\delta_m}.
		\end{gathered}
	\end{equation*}
We assumed w.l.o.g.\ that $\rode{i}{\delta_m}\geq \rode{i}{\delta_j}$ for all $j\neq i$. If $\rode{i}{\delta_m}\geq \rode{i}{\delta_i}$, then the left-hand side of the above equation is weakly negative, which is a contradiction. Therefore, $\rode{i}{\delta_i}> \rode{i}{\delta_j}$ for all $j\neq i$. Consider now the difference in the choice probability of $i$ using equation~\eqref{deg-sum} and that ${\sum_{j}\Delta\init[j]{}=0}$:
\begin{equation*}
\begin{aligned}
\rode{i}{\boldsymbol{\pi}'}-\rode{i}{\boldsymbol{\pi}}&=\Delta\init[i]{}\rode{i}{\delta_i}+\sum_{j\neq i}\Delta\init[j]{}\rode{i}{\delta_j}\\
&=-\sum_{j\neq i}\Delta\init[j]{}\rode{i}{\delta_i}+\sum_{j\neq i}\Delta\init[j]{}\rode{i}{\delta_j}\\
&=\sum_{j\neq i}\Delta\init[j]{}(\rode{i}{\delta_j}-\rode{i}{\delta_i})> 0,
\end{aligned}
\end{equation*}	
where the last inequality follows from the assumption that $\Delta\init[j]{}\leq 0$ for all $j\neq i$.

%The choice probability from a triple generated by the model has the following form
%\begin{align*}
%p(a,\{a,b,c\})&=\frac{(q_{ba}-q_{ca})(\frac{\epsilon\pi_b}{1-\epsilon}+q_{cb})+(\frac{\epsilon\pi_a}{1-\epsilon}+q_{ca})(\frac{\epsilon}{1-\epsilon}+q_{ba}+q_{bc}+q_{cb})}{(\frac{\epsilon}{1-\epsilon}+q_{ab}+q_{ac}+q_{ca})(\frac{\epsilon}{1-\epsilon}+q_{ba}+q_{bc}+q_{cb})-(q_{ba}-q_{ca})(q_{ab}-q_{cb})}.
%\end{align*}
%We compute the difference between the manipulated choice probability and the choice probability without manipulation in which the initial condition is arbitrary.
%\begin{align*}
%\Delta p(a,\{a,b,c\})&=\frac{\epsilon((1-\pi_a)\epsilon+(1-\epsilon)q_{ba}\pi_c+\pi_bq_{ca}(1-\epsilon)+(q_{bc}+q_{cb})(1-\epsilon)(1-\pi_a))}{(\frac{\epsilon}{1-\epsilon}+q_{ab}+q_{ac}+q_{ca})(\frac{\epsilon}{1-\epsilon}+q_{ba}+q_{bc}+q_{cb})-(q_{ba}-q_{ca})(q_{ab}-q_{cb})},
%\end{align*}
%which is positive for any $Q(A)$, initial distribution $\pi(A)$ and stopping time $0<\epsilon<1$
