# Supplementary material for: Markov Stochastic Choice
Source: arXiv:2410.22001 source file (2024-10-29)
Supplement: Supplementary file 5 [file app.tex]

%\section{Appendix: Proof of Proposition~\ref{prop:limit}}
\label{app1}
Fix a menu $\M\in\Mset$. We rearrange equation~\eqref{eq-def} in the following way:
\begin{align*}
\brho[b]{} &= \frac{\abs}{1-\abs} \init[]{} \left(\frac{1}{1-\abs}I-\mat[]{\M}\right)^{-1} \\
&=\frac{\abs}{1-\abs} \init[]{} \frac{1}{\text{det}\left(\frac{1}{1-\abs}I-\mat[]{\M}\right)}\text{adj}\left(\frac{1}{1-\abs}I-\mat[]{\M}\right),
\end{align*}
where adj(.) denotes the adjugate matrix. Since the Markov process is ergodic, $\mat[]{\M}$ has an eigenvalue of 1. We express the determinant with the characteristic polynomial as shown below:
\begin{align*}
\text{det}\left(\frac{1}{1-\abs}I-\mat[]{\M}\right)&=\prod_{l=1}^L \left(\frac{1}{1-\abs} -\lambda_l\right)=\frac{\abs}{1-\abs}\prod_{l=2}^L \left(\frac{1}{1-\abs} -\lambda_l\right),
%&=\left(\frac{1}{1-\abs} -1\right)\prod_{l=2}^L \left(\frac{1}{1-\abs} -\lambda_l\right)
\end{align*}
where $\lambda_l$ denotes the eigenvalues of $\mat[]{\M}$. Since $\lambda_l< 1$ for $l\neq 1$, the determinant is positive. We plug in the expression and simplify the resulting choice function
\begin{align*}
\brho[b]{} &= \init[]{} \frac{1}{\prod_{l=2}^L \left(\frac{1}{1-\abs} -\lambda_l\right)}\text{adj}\left(\frac{1}{1-\abs}I-\mat[]{\M}\right).
\end{align*}
Now we can let $\abs\rightarrow 0$:
\begin{align*}
\brho[l]{}=\lim_{\abs\rightarrow 0}\brho[b]{}&= \init[]{} \frac{1}{\prod_{l=2}^L (1 -\lambda_l)}\text{adj}(I-\mat[]{\M}).
\end{align*}
Let us multiply both sides of the equation with $(I-\mat[]{\M})$ from the right:
\begin{align*}
\brho[l]{}(I-\mat[]{\M})&= \init[]{} \frac{1}{\prod_{l=2}^L (1 -\lambda_l)}\text{adj}(I-\mat[]{\M})(I-\mat[]{\M})\\
&= \init[]{} \frac{1}{\prod_{l=2}^L (1 -\lambda_l)}\text{det}(I-\mat[]{\M})
\end{align*}
Since the matrix $(I-\mat[]{\M})$ is singular, $\text{det}(I-\mat[]{\M})=0$. Therefore,
\begin{align*}
\brho[]{}(I-\mat[]{\M})&=\boldsymbol{0}
\end{align*}
Hence, $\brho[b]{}$ converges to the unique stationary distribution of the Markov chain with transition probability matrix $\mat[]{\M}$ as $\alpha \rightarrow 0$.

%************************
\newpage
\section{Appendix: Proofs of the results on choice architecture}
\label{app-sec:choice-arch}
\subsection{Proof of Proposition~\ref{prop:attraction}}
\label{proof:attraction}
The choice probability of~$i$ in the menus $\{i,j\}$ and $\{i,j,k\}$ equals:
\begin{align*}
&\ro[c]{}{i}{i,j}=\frac{\q[c]{ji}{i,j}}{\q[c]{ji}{i,j} + \q[c]{ij}{i,j}},\\
&\ro[]{}{i}{M}=
\frac{\q{jk}{}\q{ki}{}+\q{ji}{}(\q{ki}{}+\q{kj}{})}{
\q{jk}{}\q{ki}{}+\q{ji}{}(\q{ki}{}+\q{kj}{})+\q{ij}{}(\q{jk}{}+\q{ki}{}+\q{kj}{})},
\end{align*} 
where $\M=\{i,j,k\}$. We plug the expressions in the inequality ${\ro[c]{}{i}{i,j,k}>\ro[c]{}{i}{i,j}}$ and rearrange it in the following way
\begin{equation*}
\q[c]{ij}{i,j}(\q{jk}{}\q{ki}{}+\q{ji}{}(\q{ki}{}+\q{kj}{}))>\q[c]{ji}{i,j}\q{ij}{}(\q{jk}{}+\q{ki}{}+\q{kj}{}).
\end{equation*} 
We can simplify the inequality using that $\q[c]{ji}{i,j}\q{ij}{}= \q[c]{ij}{i,j}\q{ji}{}>0$, which follows from TR-IIA, and obtain
\begin{equation*}
\begin{gathered}
\q[c]{ij}{i,j}\q{jk}{}\q{ki}{}>\q[c]{ji}{i,j}\q{ij}{}\q{jk}{}.
\end{gathered}
\end{equation*} 
We simplify the above equation, divide by $\q[c]{ij}{i,j}$ and use that $\q{ji}{}=\frac{\q[c]{ji}{i,j}\q{ij}{}}{\q[c]{ij}{i,j}}$ to get $\q{ki}{}>\q{ji}{}$.
The reverse statement can be obtained in an analogous way by assuming a \msc[l] with $\q{ki}{}>\q{ji}{}$ and showing that the choice probability of~$i$ is larger when the dominated alternative~$k$ is in the choice set.

\subsection{Proof of Proposition~\ref{prop:comparability1}}
\label{proof:comparability1}

Fix a menu $\M\in\Mset$ and an ergodic \msc[l] $\mat[]{\M}$, which is reversible on~$\M$. The \msc[l] $\mat[']{\M}$ is manipulated by comparability restrictions such that for one pair $i,j\in\M$ holds $\q{ij}{}\neq\qp{ij}{}=\qp{ji}{}=0$. We denote their respective stochastic choice functions by $\brho[l]{}$ and $\brho[l]{'}$. 

We first show that the manipulated \msc[l] is reversible on~$\M$ and ergodic. Since the non-manipulated model $\mat[]{\M}$ is reversible, it satisfies Kolmogorov's criterion on all sequences of states, i.e., for all $i_1,i_2,\dots, i_I\in\M $, 
$$\q{i_1i_2}{}\q{i_2i_3}{}\dots\q{i_{I-1}i_I}{}\q{i_Ii_1}{}=\q{i_2i_1}{}\q{i_3i_2}{}\dots\q{i_{I}i_{I-1}}{}\q{i_1i_I}{}.$$ 
Since a valid manipulation requires that the set of reachable alternatives is preserved, $\mat[']{\M}$ has to be ergodic.

Consider all sequences of alternatives in~$\M$ that do not involve~$i$ and~$j$. TR-IIA and the consistency requirement on non-manipulated pairs ensures that the model $\mat[']{\M}$ satisfies Kolmogorov's criterion on all such sequences of alternatives. Since $\qp{ij}{}=\qp{ji}{}=0$ all remaining sequences satisfy Kolmogorov's criterion trivially and the manipulated \msc[l] is also reversible on~$\M$. Since both models satisfy the detailed balance condition we have that
$$\frac{\ro[]{}{l}{\M}}{\ro[]{}{k}{\M}}=\frac{\q{kl}{}}{\q{lk}{}}=\frac{\qp{kl}{}}{\qp{lk}{}}=\frac{\ro[]{'}{l}{\M}}{\ro[]{'}{k}{\M}}\quad\quad \forall k,l\in\M\setminus\{i,j\}\text{ and }\q{lk}{}>0.$$

Next, we use the fact that rationalizable stochastic choice functions satisfy by definition the equality ${\brho[l]{}\mat[]{\M}=\brho[l]{}}$. The system can also be written as \footnote{More details can be found in the proof of Lemma~\ref{lem3} in Appendix~\ref{app-gen}.}
	\begin{equation*}
	\begin{gathered}
	\sum\limits_{\substack{k\neq l}}\ro[]{}{k}{\M}\q{kl}{}=\ro[]{}{l}{\M}\sum\limits_{\substack{k\neq l}}\q{lk}{},\\
	\sum\limits_{\substack{k\neq l}}\ro[]{'}{k}{\M}\qp{kl}{}=\ro[]{'}{l}{\M}\sum\limits_{\substack{k\neq l}}\qp{lk}{},
	\end{gathered}
	\end{equation*}
	for all $l\in\M$.
Our goal is to show $\sum\limits_{\substack{k\neq l}}\ro[]{}{k}{\M}\qp{kl}{}=\ro[]{}{l}{\M}\sum\limits_{\substack{k\neq l}}\qp{lk}{}$ for all $l\in\M$, which ensures that $\brho[l]{}$ is a stationary distribution of $\mat[']{\M}$. Set $l=i$ and consider 
	\begin{align*}
	\sum\limits_{\substack{k\neq i}}&\ro[]{}{k}{\M}\qp{ki}{}-\ro[]{}{i}{\M}\sum\limits_{\substack{k\neq i}}\qp{ik}{}=\\
	=&\sum\limits_{\substack{k\neq i\\q'_{ki}\neq 0\\q'_{ik}\neq 0}}(\ro[]{}{k}{\M}\qp{ki}{}-\ro[]{}{i}{\M}\qp{ik}{})+\sum\limits_{\substack{k\neq i\\q'_{ki}\neq 0\\q'_{ik}= 0}}\ro[]{}{k}{\M}\qp{ki}{}\\
	&-\ro[]{}{i}{\M}\sum\limits_{\substack{k\neq i\\q'_{ki}= 0\\q'_{ik}\neq 0}}\qp{ik}{}+\sum\limits_{\substack{k\neq i\\q'_{ki}=0\\q'_{ik}=0}}(\ro[]{}{k}{\M}\qp{ki}{}-\ro[]{}{i}{\M}\qp{ik}{}).
	\end{align*}
Consider the case in which $\qp{ki}{}\neq 0$ and $\qp{ik}{}=0$. The consistency assumption about the non-manipulated pairs implies that $\q{ki}{}\neq 0$ and $\q{ik}{}=0$. Detailed balance ensures that $\ro[]{}{k}{\M}=0$. This means that the second and third terms in the above expression are equal to zero. The fourth term is equal to zero trivially. We also use the assumption $\frac{\qp{ki}{}}{\qp{ik}{}}=\frac{\q{ki}{}}{\q{ik}{}}$ to modify the first term. Therefore, the resulting equation after the simplification is the following:
\begin{align*}
	\sum\limits_{\substack{k\neq i}}&\ro[]{}{k}{\M}\qp{ki}{}-\ro[]{}{i}{\M}\sum\limits_{\substack{k\neq i}}\qp{ik}{}=\\
	=&\sum\limits_{\substack{k\neq i\\q_{ki}\neq 0\\q_{ik}\neq 0}}\frac{\qp{ki}{}}{\q{ki}{}}\left(\ro[]{}{k}{\M}\q{ki}{}-\ro[]{}{i}{\M}\q{ik}{}\right).
	\end{align*}	
Since the \msc[l] $\mat{\M}$ is reversible on~$\M$, detailed balance needs to holds on all pairs. Therefore, $\ro[]{}{k}{\M}\q{ki}{}-\ro[]{}{i}{\M}\q{ik}{}=0$ for all $k\neq i$ and we have shown that the whole expression is equal to zero.

We can repeat the same argument for all other $l\in\M$. Thus, $\brho[l]{}$ is also the stationary distribution of $\mat[']{\M}$. Since the manipulated \msc[l] is irreducible, the stationary distribution of the Markov chain $\mat[']{\M}$ is unique and therefore $\brho[l]{}=\brho[l]{'}$.
 
We have now shown that restricting the comparability between a pair of alternatives does not affect the stationary distribution of the new Markov chain. If the manipulation affects more than one pair of alternatives, the argument of this proof can be applied again by taking \mat[']{\M} as the non-manipulated matrix and constructing a new manipulated matrix $\mat['']{\M}$ which does not permit the transition between a different pair of alternatives. This can be done until the actual manipulated \msc[l] is obtained.

Finally, the same argument extends trivially to the case in which the initial Markov chain is not irreducible. Since the initial distribution of the manipulated and non-manipulated \msc[l] is the same, and also because after the manipulation the decision maker is able to reach the same alternatives from each starting point as before the manipulation, the generated choice distributions of the two models are identical.

\subsection{Proof of Proposition~\ref{prop:comparability2}}
\label{proof:comparability2}
The necessity part of the argument follows directly from Proposition~\ref{prop:comparability1}. 
In order to show the sufficiency part, fix a menu $\M$ and let $\bp[n]{\M}$ be a stochastic choice function rationalizable by a \msc[l] $\mat{\M}$ and all its manipulations by comparability restrictions $\mat[']{\M}$. We consider in particular the manipulations in which the comparison between a single pair is prohibited, let this be $i,j\in\M$. It follows by the rationalizability of~$\bp[]{}$ that\footnote{More details can be found in the proof of Lemma~\ref{lem3} in Appendix~\ref{app-gen}.}
\begin{equation}
	\begin{gathered}
	\label{eq:lem}
	\sum\limits_{\substack{k\neq l}}\p{k}{\M}\q{kl}{}=\p{l}{\M}\sum\limits_{\substack{k\neq l}}\q{lk}{},\\
	\sum\limits_{\substack{k\neq l}}\p{k}{\M}\qp{kl}{}=\p{l}{\M}\sum\limits_{\substack{k\neq l}}\qp{lk}{},
	\end{gathered}
	\end{equation}
	for all $l\in\M$. Setting $l=i$ and using that $\frac{\qp{ki}{}}{\qp{ik}{}}=\frac{\q{ki}{}}{\q{ik}{}}$ and $\qp{ki}{}>0\implies \q{ki}{}>0$ for $k\neq i,j$, we can express the second inequality as follows:
	\begin{align*}
	\sum\limits_{\substack{k\neq i}}&\p{k}{\M}\qp{ki}{}-\p{i}{\M}\sum\limits_{\substack{k\neq i}}\qp{ik}{}=\\
	=&\sum\limits_{\substack{k\neq i\\q'_{ki}\neq 0}}(\p{k}{\M}\qp{ki}{}-\p{i}{\M}\qp{ik}{})-\p{i}{\M}\sum\limits_{\substack{k\neq i\\q'_{ki}= 0\\q'_{ik}\neq 0}}\qp{ik}{}= 0.
	\end{align*}
We use the assumption that $\qp{ki}{}=c\q{ki}{}$ for all $k,i\in\M$ for which comparability is not restricted and obtain
	\begin{align*}
\sum\limits_{\substack{k\neq i\\q'_{ki}\neq 0}}(\p{k}{\M}\q{ki}{}-\p{i}{\M}\q{ik}{})-\p{i}{\M}\sum\limits_{\substack{k\neq i\\q'_{ki}= 0\\q'_{ik}\neq 0}}\q{ik}{}= 0.
	\end{align*}
Since only the transition between $i$ and $j$ is restricted, the above equation becomes
	\begin{align}
	\label{eq:simplified-lem}
\sum\limits_{\substack{k\neq i,j\\q_{ki}\neq 0}}(\p{k}{\M}\q{ki}{}-\p{i}{\M}\q{ik}{})-\p{i}{\M}\sum\limits_{\substack{k\neq i,j\\q_{ki}= 0\\q_{ik}\neq 0}}\q{ik}{}= 0.
	\end{align}
	Consider now the first equation in~\eqref{eq:lem} for $l=i$:
		\begin{align*}
\sum\limits_{\substack{k\neq i,j\\q_{ki}\neq 0}}&(\p{k}{\M}\q{ki}{}-\p{i}{\M}\q{ik}{})-\p{i}{\M}\sum\limits_{\substack{k\neq i,j\\q_{ki}= 0\\q_{ik}\neq 0}}\q{ik}{}+\\ &+ \p{j}{\M}\q{ji}{}-\p{i}{\M}\q{ij}{}= 0.
	\end{align*}
	Together with~\eqref{eq:simplified-lem} this implies that detailed balance needs to be satisfied for the manipulated pair $i,j$, hence 
	\begin{align*}
\p{j}{\M}\q{ji}{}-\p{i}{\M}\q{ij}{}= 0.
	\end{align*}
	Therefore, we see that if the stochastic choice function is not susceptible to the comparability restriction of a particular pair, detailed balance is satisfied for the restricted pair. Since the stochastic choice function $\bp[n]{\M}$ is not susceptible to any manipulation, this is only possible if it holds for the rationalizing \msc[l] that detailed balance holds on all pairs, and hence that it is reversible on~$\M$.

\subsection{Proof of Proposition~\ref{prop:time}}
\label{proof:time}
Let $\M=\{i,j,k\}$ and consider the following \msc[b]s $\langle \mat[]{\M},\init[]{},\abs \rangle$ and $\langle \mat[']{\M},\init[]{},\abs \rangle$ such that $\q{ij}{}=\qp{ij}{}>0$ for all $i,j\in\M$ except $\qp[]{ik}{i,j,k}=\qp[]{ki}{i,j,k}=0$. Recall that all stochastic choice functions generated by a \msc[b] satisfy equation~\eqref{eq-def}
\begin{equation*}
	\brho[b]{} = \abs \init[]{} (I-(1-\abs)\mat[]{\M})^{-1}.
	\end{equation*}
We multiply both sides of the equation with the matrix $(I-(1-\abs)\mat[]{\M})$ and obtain the following:
\begin{equation*}
	\brho[b]{}(I-(1-\abs)\mat[]{\M}) = \abs \init[]{} =\boldsymbol{\rho}(\abs,\boldsymbol{\pi}(\M),\mat[']{\M})(I-(1-\abs)\mat[']{\M}),
	\end{equation*}
	since both models have the same stopping probability and initial distribution. We simplify the above equations in the following way
	\begin{equation}
	\label{eq:time}
	\begin{gathered}
	\brho[b]{}-\boldsymbol{\rho}(\abs,\boldsymbol{\pi}(\M),\mat[']{\M})=\\
	=(1-\abs)(\brho[b]{}\mat[]{\M}-\boldsymbol{\rho}(\abs,\boldsymbol{\pi}(\M),\mat[']{\M})\mat[']{\M}) .
	\end{gathered}
	\end{equation}
We solve the above system for \brho[b]{} and let $\brho[b]{}=\bp[]{}$ and $\boldsymbol{\rho}(\abs,\boldsymbol{\pi}(\M),\mat[']{\M})=\bp[]{}'$ to simplify the notation. We obtain the following
\begin{align*}
\p[]{i}{\M}-\pp[]{i}{\M}&=-\frac{f_i(\abs,Q)(\q{ik}{} \pp[]{i}{\M}-\q{ki}{} \pp[]{k}{\M})}{g(\abs,Q)} \text{ and }\\
\p[]{k}{\M}-\pp[]{k}{\M}&=\frac{f_k(\abs,Q)(\q{ik}{} \pp[]{i}{\M}-\q{ki}{} \pp[]{k}{\M})}{g(\abs,Q)},\\
&\text{where}\\
f_i(\abs,Q)&=(1-\abs) ((1-\abs) (\q{ji}{}+\q{jk}{}+\q{kj}{})+\abs)>0,\\
f_k(\abs,Q)&=(1-\abs) ((1-\abs) (\q{ji}{}+\q{ij}{}+\q{jk}{})+\abs)>0,\\
g(\abs,Q)&= ((1-\abs)( \q{ik}{}+ \q{ki}{})+\abs) ((1-\abs)( \q{ji}{}+ \q{jk}{})+\abs)+\\
&+(1-\abs) \q{kj}{} ((1-\abs) (\q{ji}{}+ \q{ik}{})+\abs)+\\
&+(1-\abs) \q{ij}{} ((1-\abs)( \q{ki}{}+ \q{jk}{}+\q{kj}{})+\abs)>0.
\end{align*}
Therefore, if $\q{ik}{} \pp[]{i}{\M}-\q{ki}{} \pp[]{k}{\M}<0$ it holds that $\p[]{i}{\M}-\pp[]{i}{\M}>0$ and $\p[]{k}{\M}-\pp[]{k}{\M}<0$.

If we solve~\eqref{eq:time} for $\boldsymbol{\rho}(\abs,\boldsymbol{\pi},\mat[']{\M})$ instead we obtain the following result:
\begin{align*}
\p[]{i}{\M}-\pp[]{i}{\M}&=-\frac{f_i(\abs,Q)(\q{ik}{} \p[]{i}{\M}-\q{ki}{} \p[]{k}{\M})}{g'(\abs,Q)} \text{ and }\\
\p[]{k}{\M}-\pp[]{k}{\M}&=\frac{f_k(\abs,Q)(\q{ik}{} \p[]{i}{\M}-\q{ki}{} \p[]{k}{\M})}{g'(\abs,Q)},\\
&\text{where}\\
g'(\abs,Q)&= \abs^2 + (1-\abs)(\abs(\q{jk}{}+\q{kj}{})+\q{ji}{}(\abs+(1-\abs)\q{kj}{})+\\
&+\q{ij}{}(\abs+(1-\abs)(\q{jk}{}+\q{kj}{})))>0.
\end{align*}
We make a similar conclusion that if $\q{ik}{} \p[]{i}{\M}-\q{ki}{} \p[]{k}{\M}<0$ it holds that $\p[]{i}{\M}-\pp[]{i}{\M}>0$ and $\p[]{k}{\M}-\pp[]{k}{\M}<0$.
\section{Appendix: General results on rationalizability}
\label{app-gen}
%*******************NEW
Let $\dif{ji}{}=\p{j}{\M}-\frac{\p[c]{j}{i,j}}{\p[c]{i}{i,j}}\p{i}{\M}$ for $\p[c]{i}{i,j}\neq 0$. Therefore, we can rewrite Definition~\ref{def:spo} as ${i\spo j \iff \dif{ji}{}>0}, \forall i,j\in\M.$ Here we show some auxiliary results which will be useful in the proofs of Theorems \ref{t:reversible}-\ref{t:ergodic}.
%\begin{lemma} 
%\label{lem2}
%Let $\bp{}$ be a rationalizable stochastic choice function. TR-IIA implies for all $i,j\in\M$ that
%$$\q{ij}{}\p[c]{i}{i,j}=\q{ji}{}\p[c]{j}{i,j},\quad\forall \M\in\Mset.$$
%\end{lemma}
%\begin{proof}
%The result follows directly from the definition of TR-IIA and Example~\ref{exp-binary}.
%\end{proof}
%\begin{lemma}
%\label{lem0}
%Let $\bp{}$ be a rationalizable stochastic choice function. If $\p[c]{j}{i,j}=0$ then $\q{ij}{}=0$ for all $i,j \in\M$ and $\M\in\Mset$.
%\end{lemma}
%\begin{proof}
%We know from Example~\ref{exp-binary} that $\p[c]{j}{i,j}=0$ whenever $\q[c]{ij}{i,j}=0$. By definition of the \msc[l] $\q[c]{ij}{i,j}=0$ implies that $\q[c]{ji}{i,j}\neq 0$ for all $i,j\in\M$. TR-IIA implies that $\q{ij}{}=0$.
%\end{proof}

\begin{lemma} 
\label{lem1}
Let $\bp{}$ be a stochastic choice function rationalizable by a \msc[l]. For all $i,j\in\M$ for which $\p[c]{i}{i,j}\in (0,1)$ it holds that ${\dif{ij}{}\q{ij}{}=-\dif{ji}{}\q{ji}{}}$. 
\end{lemma}
\begin{proof}
Since $\p[c]{i}{i,j}\in (0,1)$, $\q[c]{ij}{i,j}>0$ and $\q[c]{ji}{i,j}>0$. The statement is trivially satisfied for $\q{ij}{}=\q{ji}{}=0$. For $\q{ij}{}>0$ and $\q{ji}{}>0$, TR-IIA implies that $\q{ij}{}=\frac{\p[c]{j}{i,j}}{\p[c]{i}{i,j}}\q{ji}{}$.
Therefore,
	\begin{align*}
	\dif{ij}{}\q{ij}{}=&\left(\p{i}{\M}-\frac{\p[c]{i}{i,j}}{\p[c]{j}{i,j}}\p{j}{\M}\right)\frac{\p[c]{j}{i,j}}{\p[c]{i}{i,j}}\q{ji}{}\\
	=&\left(\frac{\p[c]{j}{i,j}}{\p[c]{i}{i,j}}\p{i}{\M}-\p{j}{\M}\right)\q{ji}{}\\
	=&-\dif{ji}{}\q{ji}{}.
	\end{align*}
\end{proof} 
The following lemma shows a necessary and sufficient condition for rationalizability.
\begin{lemma}
\label{lem3}
Let $\mat[]{\M}$ be a \msc[l] satisfying TR-IIA. A stochastic choice function $\bp[n]{\M}$ is rationalizable iff for all $\M \in \Mset$ it holds that
	\begin{equation}
	\label{eq:diff}
	\sum\limits_{\substack{i\neq j\\ q_{ji}\neq 0}}\dif{ji}{\M}\q{ji}{}-\sum\limits_{\substack{i\neq j\\ q_{ji}= 0}}\dif{ij}{\M}\q{ij}{}=0\quad \forall j \in \M.
	\end{equation}
\end{lemma}
\begin{proof}
	The rationalizability of $\bp{}$ implies that $\bp[n]{\M}(I-\mat[]{\M}) = 0$. Therefore, for all $j \in \M$ it holds
		\begin{equation*}
		\begin{gathered}
		\sum\limits_{\substack{i\neq j\\ q_{ij}\neq 0}}\p{i}{\M}\q{ij}{}+\p{j}{\M}\left(1-\sum\limits_{\substack{i\neq j\\ q_{ji}\neq 0}}\q{ji}{}\right)=\p{j}{\M}\\
		\sum\limits_{\substack{i\neq j\\ q_{ij}\neq 0}}\p{i}{\M}\q{ij}{}=\p{j}{\M}\sum\limits_{\substack{i\neq j\\ q_{ji}\neq 0}}\q{ji}{}\\
		\sum\limits_{\substack{i\neq j\\ q_{ji}\neq 0}}\p{j}{\M}\q{ji}{}-\sum\limits_{\substack{i\neq j\\ q_{ij}\neq 0}}\p{i}{\M}\q{ij}{}=0.
		\end{gathered}
		\end{equation*}
		We apply the TR-IIA property and obtain the following equation:
				\begin{equation*}
		\begin{gathered}
		\sum\limits_{\substack{i\neq j\\ q_{ji}\neq 0\\q_{ij}\neq 0}}\left(\p{j}{\M}-\p{i}{\M}\frac{\q[c]{ij}{i,j}}{\q[c]{ji}{i,j}}\right)\q{ji}{}-\sum\limits_{\substack{i\neq j\\q_{ji}= 0\\ q_{ij}\neq 0}}\p{i}{\M}\q{ij}{}+\sum\limits_{\substack{i\neq j\\ q_{ji}\neq 0\\q_{ij}= 0}}\p{j}{\M}\q{ji}{}=0.
		\end{gathered}
		\end{equation*}
	We know from Example~\ref{exp-binary} that the ratio of transition probabilities for binary sets is equal to the choice probability ratio. We can rewrite the above equality using function $d()$ as shown below and obtain the final result:
				\begin{equation*}
		\begin{gathered}
		\sum\limits_{\substack{i\neq j\\ q_{ji}\neq 0\\q_{ij}\neq 0}}\dif{ji}{}\q{ji}{}-\sum\limits_{\substack{i\neq j\\q_{ji}= 0\\ q_{ij}\neq 0}}\dif{ij}{}\q{ij}{}+\sum\limits_{\substack{i\neq j\\ q_{ji}\neq 0\\q_{ij}= 0}}\dif{ji}{}\q{ji}{}=0\\
		\sum\limits_{\substack{i\neq j\\ q_{ji}\neq 0}}\dif{ji}{}\q{ji}{}-\sum\limits_{\substack{i\neq j\\q_{ji}= 0}}\dif{ij}{}\q{ij}{}=0.
		\end{gathered}
		\end{equation*}
\end{proof}
%************************
\section{Appendix: Proofs of the characterization results of reversible limiting MSC models}
\label{app-luce}

\subsection{Proof of Theorem~\ref{t:reversible}}
\label{proof:theorem-reversible}

\textit{Necessity}: Fix a menu $\M\in\Mset.$ We consider a \msc[l] \mat[]{\M} with generated stochastic choice function $\brho{}=\bp[n]{\M}$. We will show that if a \msc[l] violates reversibility on~$M$, the generated stochastic choice function $\bp[n]{\M}$ is cyclical.

The proof is structured as follows. First, we show that a \msc[l], which is not reversible on~$\M$, generates stochastic choice functions which satisfy $\spo\neq\emptyset$. Then, we represent the equations in~\eqref{eq:diff} in matrix notation for each menu. If the Markov chain is not reversible on~$\M$, the system has a positive solution. We invoke Gordan's theorem, which gives a necessary and sufficient condition for the existence of positive solutions to a homogeneous linear system and show the relationship of the condition to the cyclicity property of $\spo$. 

If a \msc[l] is not reversible on~$\M$, then detailed balance is violated for at least one pair $i,j\in\M$, hence: 
\begin{equation}
\q{ij}{}\p{i}{\M}\neq\q{ji}{}\p{j}{\M}.
\label{eq:violation-rev}
\end{equation}
Assume by contradiction that $\spo=\emptyset$. This means that it holds for $i,j$ that
\begin{equation}
\p[c]{j}{i,j}\p{i}{\M}=\p[c]{i}{i,j}\p{j}{\M}.
\label{eq:spo-empty}
\end{equation}
If $\p{i}{\M}=\p{j}{\M}=0$, then inequality~\eqref{eq:violation-rev} is violated. If $\p{i}{\M}>0,\p{j}{\M}=0$, equation~\eqref{eq:spo-empty} implies that $\p[c]{i}{i,j}=0$ and hence $\q[c]{ji}{i,j}=0$. It follows from TR-IIA that $\q{ji}{}=0$, which would then violate~\eqref{eq:violation-rev}. Finally, if $\p{i}{\M}>0,\p{j}{\M}>0$ implies together with~\eqref{eq:spo-empty} that $\p[c]{j}{i,j}>0$ and $\p[c]{i}{i,j}>0$. This in turn means that $\q[c]{ji}{i,j}=0$ and $\q[c]{ij}{i,j}=0$. TR-IIA is satisfied when either $\q{ij}{}=\q{ji}{}=0$ or when both are strictly positive and 
\begin{equation*}
\frac{\p{j}{\M}}{\p{i}{\M}}=\frac{\p[c]{j}{i,j}}{\p[c]{i}{i,j}}=\frac{\q[c]{ji}{i,j}}{\q[c]{ij}{i,j}}=\frac{\q{ji}{}}{\q{ij}{}}.
\end{equation*}
Both of these cases violate~\eqref{eq:violation-rev}. Therefore, if a \msc[l] is not reversible on~$\M$ then $\spo\neq\emptyset$.

Recall that $\dif{ji}{}=\p{j}{\M}-\frac{\p[c]{j}{i,j}}{\p[c]{i}{i,j}}\p{i}{\M}$ for $\p[c]{i}{i,j}\neq 0$ as defined in Appendix~\ref{app-gen}. Let $f_{\M}:\M\rightarrow[1,\dots , |\M|]$ be a bijective mapping assigning an index to each alternative in the menu $\M$. Further, we denote by $\G$ a set of ordered pairs in the menu such that for all $i,j\in\M$, $(i,j)\in\G$ unless $\ro[c]{}{j}{i,j}=0$ or $(j,i)\in\G$ or $\dif{ij}{}=0$. Note that since there is some $i,j\in\M$ for which $\dif{ij}{}\neq 0$, $\G\neq\emptyset$. We denote with $\g:\G\rightarrow[1,\dots , |\G|]$ a bijective mapping on the set of ordered pairs. Further, we define a vector of transition probabilities $\sav$ between the pairs in $\G$, that is $\gamma_{\g[i,j]}
(\M)=\q{ij}{}$. Finally, we denote by $\mathcal{D}(\M)$ a
%${|M|\times \frac{|M||M-1|}{2}}$
 matrix with dimensions $|\M|\times|\G|$ and elements
 \begin{align*}
\difel{f_{\M}(k)}{\g[i,j]}=\begin{cases}
\dif{ij}{}, &\text{ if } k=i,\\
-\dif{ij}{}, &\text{ if } k=j,\\
0 &\text{ if }k\neq i, k\neq j,
\end{cases}
\end{align*}
where $k\in\M$ and $(i,j)\in\G$. Note that all elements of the matrix  given by the functions $\dif{ij}{}$ are defined since if $\ro[c]{}{j}{i,j}=0$, $(i,j)\not\in\G$. Further, none of the columns of the matrix are equal to $\textbf{0}$ because if $\dif{ij}{}=0$, $(i,j)\not\in\G$. 
We claim that the system
	\begin{equation}
	\label{eq:diff-system}
	\mathcal{D}(\M)\sav{}=\boldsymbol{0} 
	\end{equation}
is equivalent to the one in~\eqref{eq:diff} and is thus necessary and sufficient for rationalizability. In order to verify this claim, we consider an equation from the system in~\eqref{eq:diff-system} corresponding to an arbitrary matrix row $f_{\M}(j)$:
	\begin{equation*}
	\begin{gathered}
\sum\limits_{\substack{i\in\M\\ (j,i)\in \G}}\difel{f_{\M}(j)}{\g[j,i]}\gamma_{\g[j,i]}(\M)+ \sum\limits_{\substack{i\in\M\\ (i,j)\in \G}}\difel{f_{\M}(j)}{\g[i,j]}\gamma_{\g[i,j]}(\M)=0\\
 \sum\limits_{\substack{i\in\M\\ (j,i)\in \G}}\dif{ji}{}\q{ji}{}-\sum\limits_{\substack{i\in\M\\ (i,j)\in \G}}\dif{ij}{}\q{ij}{}=0\\
\sum\limits_{\substack{i\neq j\\ q_{ji}\neq 0}}\dif{ji}{\M}\q{ji}{}-\sum\limits_{\substack{i\neq j\\ q_{ji}= 0}}\dif{ij}{\M}\q{ij}{}=0,
	\end{gathered}
	\end{equation*}
	where we obtain the last equation by applying Lemma~\ref{lem1} and letting $\dif{ij}{\M}\q{ij}{}=-\dif{ji}{\M}\q{ji}{}$ for all $(i,j)\in \G$ for which $\q{ji}{}\neq 0$. For all such pairs for which $\q{ji}{}>0$, TR-IIA implies that $\q[c]{ji}{i,j}>0$ and hence, $\p[c]{i}{i,j}>0$, which ensures that $\dif{ji}{\M}$ is defined. 
%	
%If the \msc[l] \mat{\M} is reversible, then for each pair $i,j$ we either have $\dif{ij}{}=0$ or/and $\q{ij}{}=\q{ji}{}=0$. Therefore, reversible models correspond to the solution $\sav{}=\boldsymbol{0}$ of the system~\eqref{eq:diff-system}. Since this is a trivial solution, reversible \msc[l] can generate all stochastic choice functions. On the other hand, 

If the \msc[l] is non-reversible on~$\M$, there must be at least one pair $i,j$ for which $\dif{ij}{}\neq 0$ and $\q{ij}{}>0$ and/or $\q{ji}{}>0$, which means that $\sav{}\geq \boldsymbol{0}$. We apply Gordan's theorem\footnote{See for example Theorem 15.1(2) in \citeA{Woerdeman2015}.} which states that there exists a strictly positive solution ${\sav{}\geq \boldsymbol{0}}$ to the linear system in~\eqref{eq:diff-system} if and only if there does not exist a vector $\boldsymbol{v}\in\mathbb{R}^{|M|}$ for which
\begin{equation}
\label{eq:sys-strongly1}
\boldsymbol{v}\mathcal{D}(\M)\gg\boldsymbol{0}.
\end{equation}
Let us denote the elements of the vector $\boldsymbol{v}=(v_i,v_j,\dots)$ such that $\boldsymbol{v}_{f_{\M}(i)}=v_i$. The linear system in~\eqref{eq:sys-strongly1} is equivalent to
\begin{equation*}
v_i\difel{f(i)}{\g[i,j]} + v_j\difel{f(j)}{\g[i,j]}>0, \quad \forall (i,j) \in \G,
\end{equation*}
which is in turn equal to
\begin{equation}
\label{eq:v-diff}
(v_i - v_j)\dif{ij}{\M}>0, \quad \forall (i,j) \in \G.
\end{equation}
Hence, each inequality in~\eqref{eq:v-diff} specifies whether $v_i>v_j$ or $v_j>v_i$ depending on the sign of $\dif{ij}{}$ for all $(i,j) \in\G$ (recall that for all $(i,j) \in\G$, $\dif{ij}{}\neq 0$). As we argued above, if the Markov chain is non-reversible on~$\M$, the system in \eqref{eq:diff-system} has a strictly positive solution, and hence there does not exist a vector $\boldsymbol{v}$ satisfying \eqref{eq:v-diff}. 
This is the case when the elements of $\M'\subseteq\M$ can be ordered in a sequence $(i_1,i_2,\dots,i_I)$ such that ${\dif{i_1i_2}{}>0},{\dif{i_2i_3}{}>0,\dots},{\dif{i_{I-1}i_I}{}>0},{\dif{i_{I}i_1}{}>0}$. Combining this insight with the definition of the binary relation $\spo$ implies that \spo is cyclical.

\textit{Sufficiency}: The sufficiency part of the proof has a similar structure to the necessity proof. Fix a menu $\M\in\Mset$.
We first consider the case in which $\spo=\emptyset$, therefore 
\begin{equation}
\label{eq:revers-bin1}
\p[c]{j}{i,j}\p{i}{\M}=\p[c]{i}{i,j}\p{j}{\M},\quad \forall i,j\in\M.
\end{equation}
This means that $\dif{ij}{}=0$ for all $i,j\in\M$ for which it is defined. Lemma~\ref{lem3} implies that there exists a \msc[l] that rationalizes it. We now show that it is reversible on~$\M$. Consider an arbitrary pair $i,j\in\M$.
If $\p[c]{i}{i,j}\p{j}{\M}>0$ then necessarily $\p[c]{j}{i,j}>0$ and $\p{i}{\M}>0$. This in turn implies that $\q[c]{ij}{i,j}>0$ and $\q[c]{ji}{i,j}>0$. If $\q{ij}{}=\q{ji}{}=0$, detailed balance is satisfied trivially. It is not possible that $\q{ij}{}>0$ and $\q{ji}{}=0$ or vice versa, because it would violate TR-IIA. If both $\q{ij}{}>0$ and $\q{ji}{}>0$ it holds that
\begin{equation*}
\frac{\p{j}{\M}}{\p{i}{\M}}=\frac{\p[c]{j}{i,j}}{\p[c]{i}{i,j}}=\frac{\q{ji}{}}{\q{ij}{}}
\end{equation*}
and detailed balance is satisfied on the pair. If $\p[c]{i}{i,j}\p{j}{\M}=0$ and $\p{i}{\M}=0$ there are two possible subcases: $\p[c]{i}{i,j}=0$ or/and $\p{j}{\M}=0$. Detailed balance is trivially satisfied in the latter. In the former case, $\p[c]{i}{i,j}=0$ implies that $\q[c]{ji}{i,j}=0$. Using TR-IIA we get that $\q{ji}{}=0$ and detailed balance is again satisfied. Analogously, if $\p{j}{\M}=0$ and $\p[c]{j}{i,j}=0$, detailed balance is satisfied. We can conclude that in the case when $\spo=\emptyset$ the rationalizing model is reversible on~$\M$. We will assume for the remainder of the proof that $\spo\neq\emptyset$.

In the second part of the proof, we start by creating the matrix $\mathcal{D}(\M)$ and use Gordan's theorem, similarly to the necessity proof. If \spo is cyclical, there is a strictly positive solution to the system in~\eqref{eq:diff-system} and if it is acyclical, the only non-negative solution is the zero vector. Using the solution to the homogeneous system, we can create transition probability matrices such that TR-IIA is satisfied and $\bp{}$ is a left eigenvector.

Let $\bp{}$ be a stochastic choice function such that $\spo\neq\emptyset$. 
Fix a menu $\M$ and define the set $\G$ and the functions $f_{\M}(.)$ and $\g[.]$ as shown in the necessity part of the proof. We also define the matrix $\mathcal{D}(\M)$ analogously. If \spo is acyclical there is a vector  $\boldsymbol{v}\in\mathbb{R}^{|M|}$ for which
\begin{equation}
\label{eq:sys-strongly}
\boldsymbol{v}\mathcal{D}(\M)\gg\boldsymbol{0}.
\end{equation} 
On the contrary, if \spo is cyclical, there is no such vector.
Applying Gordan's theorem we know that the system 
\begin{equation}
	\label{eq:diff-system2}
	\mathcal{D}(\M)\sav{}=\boldsymbol{0}
	\end{equation}
has a strictly positive solution if \spo is cyclical and no strictly positive solution if \spo is acyclical.

We can now use the solution to the above system to construct a transition probability matrix $\mat[]{\M}$. In particular, we define
\begin{align}
\q{ij}{}=\begin{cases} 
\gamma_{\g[i,j]}& \text{ if }(i,j)\in\G,\\
0 & \text{ if }\p[c]{j}{i,j}=0,\\
(0,1)& \text{ if }\dif{ij}{i,j}=0.
\end{cases}
\label{qij}
\end{align}

 We then let 
\begin{align}
\q{ji}{}=\begin{cases} 
\q{ij}{}\frac{\p[c]{i}{i,j}}{\p[c]{j}{i,j}}& \text{ if }(i,j)\in\G \text{ or }\dif{ij}{}=0,\\
0 & \text{ if }\p[c]{i}{i,j}=0,\\
(0,1)& \text{ if }\dif{ji}{}=0\text{ and }\p[c]{j}{i,j}=0.\\
\end{cases}
\label{qji}
\end{align}
We ensure that $\sum_{j\neq i}\q{ij}{}< 1$ by scaling down all non-diagonal entries in the matrix by the same factor. Finally, we let $\q{ii}{}=1-\sum_{j\neq i}\q{ij}{}$.

Note that the constructed matrix satisfies trivially TR-IIA for all pairs $i,j$ for which $\p[c]{i}{i,j}\neq 0$. Also if $\p[c]{i}{i,j}=0$ this implies that $\q[c]{ji}{i,j}=0$. Since then $\q{ji}{}=0$, TR-IIA is satisfied as well.

Since the systems~\eqref{eq:diff-system2} and~\eqref{eq:diff} are equivalent, Lemma~\ref{lem3} implies that the stochastic choice function is rationalizable with the constructed \msc[l] on~$\M$. The procedure can be repeated analogously on all~$\M\in\Mset$.
\subsection{Proof of Corollary~\ref{cor:metro}}
\label{proof:metropolis}
We show that among the rationalizing models there is always going to be a model with symmetric relative salience parameters by letting $\tr{ij}=\p[c]{j}{i,j}$ for all $i,j\in\all$. We then generate the rationalizing \msc[l] from choice data analogously as shown in the proof of Theorem~\ref{t:reversible}. If $\q{ij}{}=\q{ji}{}=0$, then $\sa{ij}{}=\sa{ji}{}=0$. Having $\q{ij}{}>0$ and $\q{ji}{}=0$ implies $\q[c]{ji}{i,j}=0$ and $\tr{ji}=0$. We can then let $\sa{ji}{}=\sa{ij}{}$. Finally, if $\q{ij}{}>0$ and $\q{ji}{}>0$, TR-IIA implies that $\sa{ji}{}=\sa{ij}{}\frac{\tr{ij}}{\tr{ji}}\frac{\p[c]{i}{i,j}}{\p[c]{j}{i,j}}=\sa{ij}{}$. Therefore, the constructed model rationalizes the choice data and has symmetric relative salience parameters.

\section{Appendix: Proofs of Theorems~\ref{t:all} and~\ref{t:ergodic}}
\label{app-t23}
\subsection{Proof of Theorem~\ref{t:all}}
\label{proof:theorem-all}
\textit{Necessity}: Let $\mat[]{\M}$ be a \msc[l] with no $i,j\in\M$ for which $\q{ij}{}=\q{ji}{}=0$ for all $\M\in\Mset$. Assume by contradiction that there is a choice set $\M\in\Mset$ and a pair $k,l\in\M$ which violates the\btc{m}. This is the case when $k\spo l$ and there is no cycle such that $(k,l)\in\cy$. This assumption implies that $\spo\neq \emptyset$. We construct the set $\G$, the matrix $\mathcal{D}(\M)$ and the vector $\sav{}$ as shown in the proof of Theorem~\ref{t:reversible}. Since there is no $i,j\in\M$ for which $\q{ij}{}=\q{ji}{}=0$, $\sav{}\gg\boldsymbol{0}$. We use Stiemke's lemma, which states that there exists a strongly positive solution $\sav{}$ to the linear system in~\eqref{eq:diff-system} if and only if there does not exist a vector $\boldsymbol{v}\in\mathbb{R}^{|M|}$ for which
\begin{equation}
\label{eq:sys-strongly-ii}
\boldsymbol{v}\mathcal{D}(\M)\geq\boldsymbol{0}.
\end{equation}
Analogously to~\eqref{eq:v-diff}, this system can be written as
\begin{equation*}
\label{eq:v-diff1}
(v_i - v_j)\dif{ij}{\M}\geq 0, \forall (i,j) \in \G \text{ and } (v_i - v_j)\dif{ij}{\M}> 0 \text{ for at least one }(i,j) \in \G.
\end{equation*}
Since $\sav{}\gg\boldsymbol{0}$, such vector $\boldsymbol{v}$ does not exist. However, since $(k,l)\not\in\cy$, one can set $v_l>v_k$ and therefore $(v_k - v_l)\dif{kl}{\M}> 0$, which is a contradiction. Therefore, only when it holds for all pairs of alternatives $(i,j)\in \G$ that there is some cycle \cy such that $(i,j)\in\cy$, we can ensure that $v_i=v_j$ for all $(i,j)\in\G$.

If the \msc[l] is such that $\q{ij}{}>0$ for all $\M\in\Mset$ and all $i,j\in\M$, this means that $\q[c]{ij}{i,j}>0$ for all $i,j\in\all$. Therefore, it holds that $\ro[c]{}{i}{i,j}>0$ for all $i,j\in\all$.

\textit{Sufficiency}: 
%\begin{lemma}
%If all pairs of alternatives are\btc{}, then the stochastic choice function is positive on~$\M$.
%\end{lemma}
%\begin{proof}
%Assume by contradiction that there is $i\in\M$ with $\p{i}{\M}=0$. Alternative~$i$ cannot be part of a cycle since $\dif{ji}{}\geq 0$ for all $j\neq i$. The\btc{c} implies that we should have $(i,j)\not\in\spo$ and $(j,i)\not\in\spo$ for all $j\neq i$.
%\end{proof}
We now show that if choice over all pairs of alternatives in all menus is\btc{}, there always exists a rationalizing \msc[l] such that there is no $i,j\in\M$ for which $\q{ij}{}=\q{ji}{}=0$ for all $i,j\in\M$. We construct the set $\G$, the matrix $\mathcal{D}(\M)$ and the vector $\sav{}$ as shown in the proof of Theorem~\ref{t:reversible}. We use Stiemke's lemma, which states that there exists a strongly positive solution to the linear system in~\eqref{eq:diff-system2} if and only if there does not exist a vector $\boldsymbol{v}\in\mathbb{R}^{|M|}$ for which
\begin{equation}
\label{eq:sys-strongly2}
\boldsymbol{v}\mathcal{D}(\M)\geq\boldsymbol{0}.
\end{equation}
We can alternatively write this linear system as
\begin{equation*}
\label{eq:v-diff2}
(v_i - v_j)\dif{ij}{\M}\geq 0, \forall (i,j) \in \G \text{ and } (v_i - v_j)\dif{ij}{\M}> 0 \text{ for at least one }(i,j) \in \G.
\end{equation*}
We will show that the assumption that all pairs of alternatives are\btc{} implies that there is no pair $(i,j)\in\G$ for which $(v_i - v_j)\dif{ij}{\M}> 0$. Since all pairs of alternatives are\btc{}, it holds for all $(i,j)\in\G$, that there exist a cycle $\cy$ such that $(i,j)\in\cy$, where $\M'\subseteq\M$ might be different for some pairs in the set. The inequality~\eqref{eq:v-diff2} implies that for all alternatives $\{i_1',i_2',\dots,i_I'\}$ belonging to a cycle on $\M'$ it holds that $v_{i_1'}=v_{i_2'}=v_{i_3'}=\dots=v_{i_I'}$. It holds, therefore, that $(v_i - v_j)\dif{ij}{\M}= 0$ for all $(i,j)\in\cy$. The only possible way of having a pair $(i,j)\in\G$ for which $(v_i - v_j)\dif{ij}{\M}> 0$ is that $i$ and~$j$ do not belong to the same cycle. However, if that is true, the\btc{c} would imply that $(i,j)\not\in\spo$ and $(j,i)\not\in\spo$, which in turn implies that $(i,j)\not\in\G$. This means, however, that $\boldsymbol{v}\mathcal{D}(\M)=\boldsymbol{0}$. Therefore, the\btc{c} implies that the solution of the system~\eqref{eq:diff-system2} is strongly positive. We construct a transition probability matrix $\mat{\M}$ as shown in the proof of Theorem~\ref{t:reversible}. Note in particular that it holds for all pairs $(i,j)\not\in\G$ that $\q{ij}{}>0$ unless $\p[c]{j}{i,j}=0$ following the proposed construction of the stochastic choice function. This is the case since the\btc{c} implies positivity of the stochastic choice function of $\M$. The constructed Markov chain rationalizes $\bp[]{}$ and satisfies TR-IIA. 

If the stochastic choice function is positive for all binary menus, we can immediately see from the construction of the transition probability matrix that all entries will be strictly positive.

\section{Proofs of the identification results}
\label{app-zerotr}
%We assume by contradiction that a stochastic choice in which some pair $i,j\in\M$ is not\btc{} can be rationalized by a \msc[l] with $\q{ij}{}>0$ and show that this cannot be the case. Since choice over the pair~$i$ and~$j$ is not\btc{}, Theorem~\ref{t:ergodic} guarantees that in the model there is at least one pair $k,l\in\M$ with $k\spo l$ for which $\q{kl}{}=\q{lk}{}=0$. We show the contradiction by constructing stochastic choice functions $\bp{}'$ from $\bp{}$ for each set of possible zero probability transitions in the rationalizing model by adjusting $\p[c]{k}{k,l}$ such that $\dif{kl}{}'=0$ for all $\q{kl}{}=0$. These stochastic choice functions are rationalizable by models with $\q{mn}{}'=\q{mn}{}\neq 0$ and $\q{mn}{}'\in(0,1)$ for $\q{mn}{}=0$. Therefore, for the constructed stochastic choice function in which the set of manipulated pairs overlaps with the set in which the rationalizing model $\mat{\M}$ has a zero probability transition, there must exist a rationalizing model with strictly positive transitions. Theorem~\ref{t:ergodic} implies that this is the case if all pairs are\btc{}. Since $i$ and $j$ do not belong to the same cycle in $\bp{}$, they also do not belong to the same cycle in any of the constructed stochastic choice functions, therefore we must have $\q{ij}{}=0$.

\subsection{Proof of Proposition~\ref{prop:salience}}
\label{proof:salience}

We start by recalling a result in Lemma~\ref{lem3} in Appendix~\ref{app-gen}, which follows directly from the definition of rationalizable stochastic choice functions with the \msc[l]
	\begin{equation*}
	\begin{gathered}
	\sum\limits_{\substack{j\neq i}}\p{j}{\M}\q{ji}{}=\p{i}{\M}\sum\limits_{\substack{j\neq i}}\q{ij}{}.
		\end{gathered}
	\end{equation*}
	We simplify the above equation, using that $\M=\{i,j,k\}$ and that $\q{ij}{}\neq 0$ for all $i,j\in\M$ and obtain: 
	\begin{equation*}
	\begin{gathered}
	(\p{i}{\M}\q{ij}{}-\p{j}{\M}\q{ji}{})+(\p{i}{\M}\q{ik}{}-\p{k}{\M}\q{ki}{})=0.
	\end{gathered}
	\end{equation*}
We use Proposition~\ref{binary-identification} and substitute $\q{ij}{}=\sa{ij}{}\p[c]{j}{i,j}=\sa{ji}{}\p[c]{j}{i,j}$ for all $i,j\in\M$ and obtain
	\begin{equation*}
	\begin{gathered}
	\frac{\sa{ij}{}}{\sa{ik}{}}=\frac{\p{k}{\M}\p[c]{i}{i,k}-\p{i}{\M}\p[c]{k}{i,k}}{\p{i}{\M}\p[c]{j}{i,j}-\p{j}{\M}\p[c]{i}{i,j}}.
		\end{gathered}
	\end{equation*}

	We have that $\sa{ij}{}>\sa{ik}{}$ if 
		\begin{equation*}
	\begin{gathered}
	\frac{\p{k}{\M}\p[c]{i}{i,k}-\p{i}{\M}\p[c]{k}{i,k}}{\p{i}{\M}\p[c]{j}{i,j}-\p{j}{\M}\p[c]{i}{i,j}}>1.\\
		\end{gathered}
	\end{equation*}
We can now factor out $\p{i}{\M}\p[c]{i}{i,k}$ from the nominator and $\p{i}{\M}\p[c]{i}{i,j}$ from the denominator to obtain the following inequality:
	\begin{equation*}
	\begin{gathered}
	\frac{\p{i}{\M}\p[c]{i}{i,k}\left(\frac{\p{k}{\M}}{\p{i}{\M}}-\frac{\p[c]{k}{i,k}}{\p[c]{i}{i,k}}\right)}{\p{i}{\M}\p[c]{i}{i,j}\left(\frac{\p[c]{j}{i,j}}{\p[c]{i}{i,j}}-\frac{\p{j}{\M}}{\p{i}{\M}}\right)}>1.
	\end{gathered}
	\end{equation*}
We can cancel out the term $\p{i}{\M}$ and rearrange to obtain the final result.
